# Supplementary material for: Boundedness of varieties of Fano type with alpha-invariants and volumes bounded below
Source: arXiv:1810.04019 source file (2018-10-23)
Supplement: Supplementary file 1 [file appendix.tex]

\section{On rationally connectedness of varieties of CY-type}\label{appendix}

The goal of this appendix is to give a sufficient condition for a dlt log Calabi--Yau pair being rationally connected. It was suggested by Chenyang Xu and carried out during a discussion with Zhiyu Tian.

Given a log pair $(X, B)$, recall that a subvariety $C\subset X$ is said to be a {\it log center} or {\it non-canonical center}  if there is a prime divisor $E$ over $X$ with center $C$ such that the log discrepancy $a(E, X, B)<1$.

The following is the main result of this appendix.

\begin{thm}\label{thm:dltcyrc}
Let $(X,B)$ be an lc log Calabi--Yau pair with a log center $C$, % which is rationally chain connected, 
then $X$ is rationally chain connected modulo $C$.
In particular, if $C$ is rationally chain connected, then  $X$ is rationally chain connected.
\end{thm}

As a simple corollary, we have the following interesting result. %which was a question asked by the first author.
\begin{cor}\label{cor:dltcydisrc}
Let $(X,B)$ be a dlt log Calabi--Yau pair with a $0$-dimensional log center. Then  $X$ is rationally connected.
\end{cor}

%Using a similar argument of the proof of Theorem \ref{thm:dltcyrc}, we get a sufficient condition on lc log Calabi--Yau pairs to be rationally chain connected.   
%\begin{thm}\label{thm:lccyrc}
%	Let $(X,B)$ be a lc log Calabi--Yau pair. If $(X,B)$ has a log center $C$ which is rationally chain connected, then $X$ is rationally chain connected. 
%\end{thm}

\begin{proof}[Proof of Theorem \ref{thm:dltcyrc}]
By assumption, there exists a prime divisor $E$ over $X$, such that the center of $E$ on $X$ is $C$, and $a:=a(E,X,B)<1$. By \cite[Corollary 1.4.3]{BCHM}, after taking a dlt modification of $(X, B)$, there exists a birational morphism $f:X'\to X$, such that
$$K_{X'}+B'+(1-a)E=f^{*}(K_X+B)\equiv0,$$
where $B'$ is the sum of the birational transform of $B$ on $X'$ and the exceptional divisors of $f$ except for $E$. It suffices to show that $X'$ is rationally chain connected modulo $E$.% If this is the case, $X$ is rationally chain connected modulo $C$, hence $X$ is rationally chain connected. By \cite[Corollary 1.8]{HM}, $X$ is rationally connected.

Run a $(K_{X'}+B')$-MMP with scaling of an ample divisor on $X'$, according to \cite[Corollary 1.3.3]{BCHM}, the MMP ends up with a Mori fiber space $ Y\to Z$.
	$$\xymatrix@=2.5em{
	&        W  \ar[dl]_{p}  \ar[dr]^{q}                &\\	
	X'\ar@{-->}[rr]^{\pi}\ar[d]^{f}  & &   Y\ar[d]^{g}\\
	X         &  &Z\\
}
$$ 
Let $W\subset X'\times Y$ be the closure of the graph of $\pi$, and $p$ and $q$ are the projections from $W$ to $X'$ and $Y$, respectively. Since $-K_Y$ is ample over $Z$ and $Y$ is klt,  according to \cite[Theorem 1.2]{hm07}, every fiber of $W\to Z$ is rationally chain connected. 

Let $E_Y,E_W$ be the birational transform of $E$ on $Y$ and $W$, respectively. Since the MMP is also a $(-E)$-MMP, $E_Y$ dominates $Z$. Thus, $W$ is rationally chain connected modulo $E_W$, and hence $X'$ is rationally chain connected modulo $E$. We complete the proof.
\end{proof}
\begin{proof}[Proof of Corollary \ref{cor:dltcydisrc}]
	Follows easily from Theorem \ref{thm:dltcyrc} and \cite[Corollary 1.5(2)]{hm07}.
\end{proof}
